# Supplementary material for: Machine learning-based detection of cardiovascular disease using ECG signals: performance vs. complexity
Source: arXiv:2303.11429 source file (2023-03-10)
Supplement: Supplementary file 1 [file appendix.tex]

\chapter{Dataset Examples}

\begin{figure}[h]
    \centering
    \includegraphics[width=\textwidth]{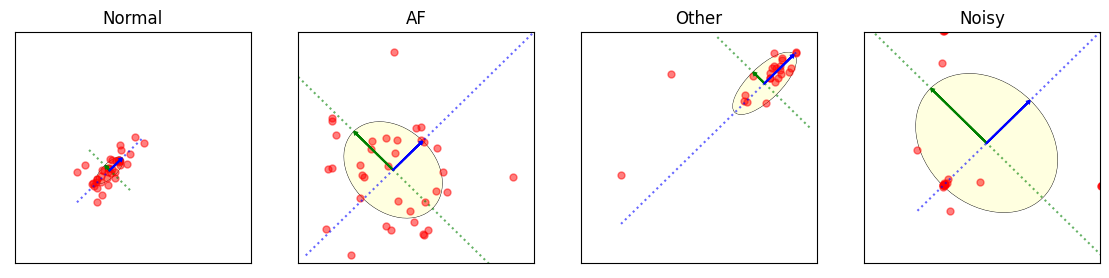}
    \caption{The examples of each class in CinC 2017 dataset}
    \label{fig:cinc2017_classes}
\end{figure}

\begin{figure}[h]
    \centering
    \includegraphics[width=0.9\textwidth]{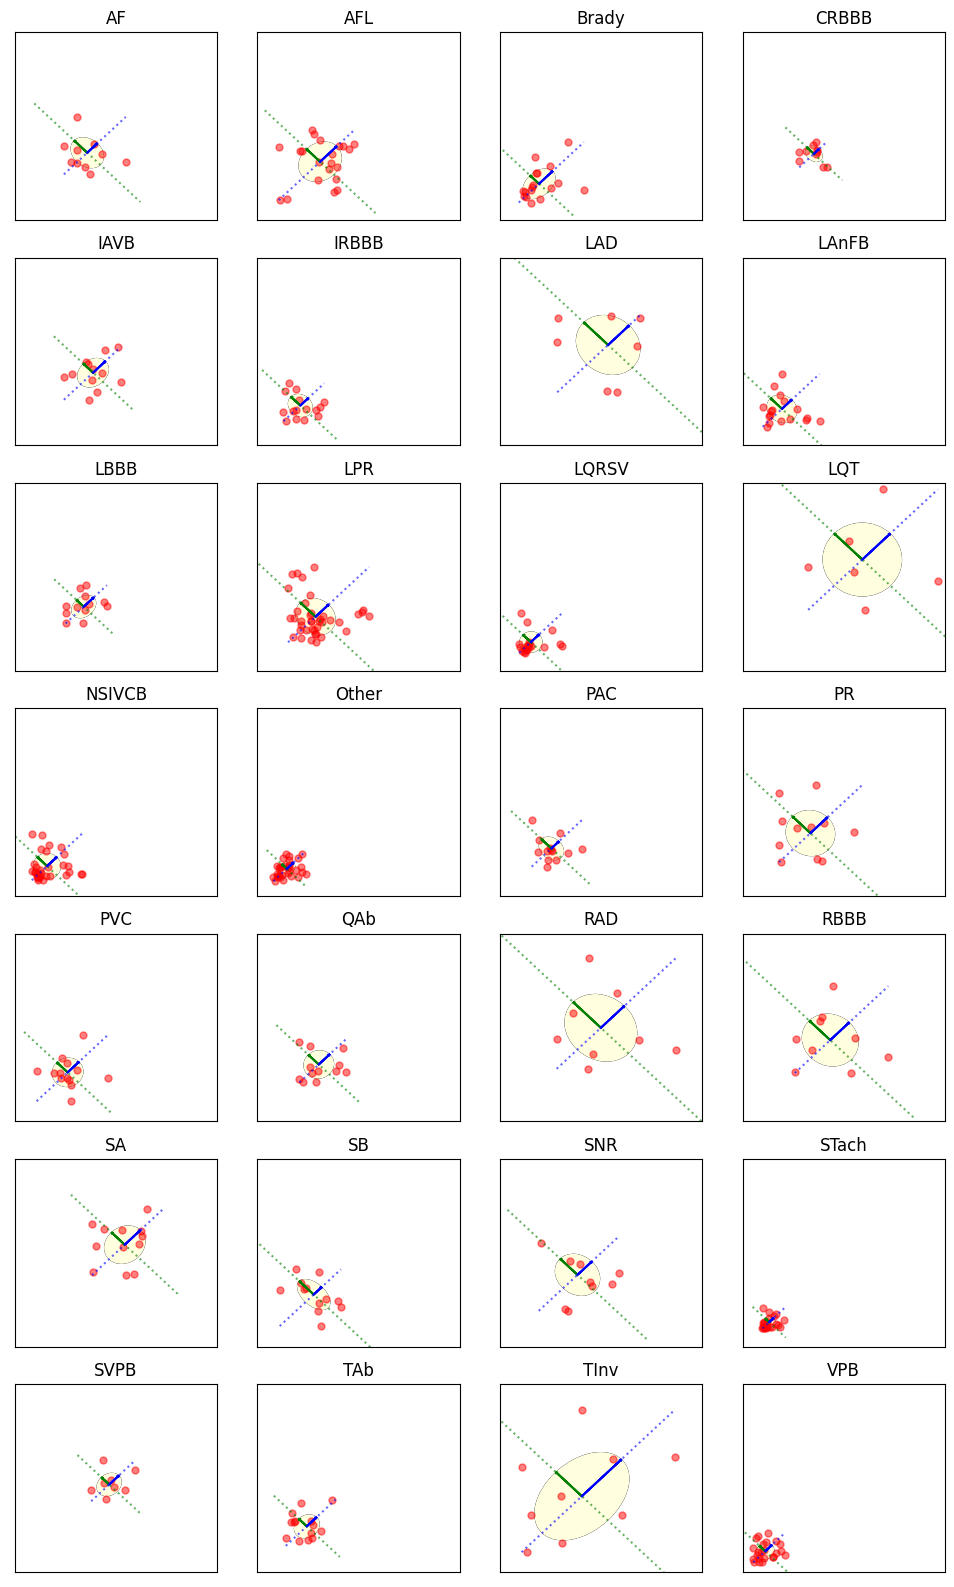}
    \caption{The examples of each class in CinC 2020 dataset}
    \label{fig:cinc2020_classes}
\end{figure}

\chapter{Classification Report}
\section{CinC 2017}

\begin{table}[h]
    \centering
    \begin{tabular}{|l|r|r|r|r|}
    \hline
    \textbf{Classes} & \textbf{Precision} & \textbf{Recall} & \textbf{F1 Ccore} & \textbf{Support} \\ \hline
    N & 0.84 & 0.85 & 0.84 & 1044 \\ \hline
    A & 0.79 & 0.41 & 0.54 & 140 \\ \hline
    O & 0.6 & 0.39 & 0.47 & 473 \\ \hline
    $\sim$ & 0.00 & 0.00 & 0.00 & 49 \\ \hline
    micro avg & 0.78 & 0.66 & 0.72 & 1706 \\ \hline
    macro avg & 0.56 & 0.41 & 0.46 & 1706 \\ \hline
    weighted avg & 0.74 & 0.66 & 0.69 & 1706 \\ \hline
    samples avg & 0.65 & 0.66 & 0.66 & 1706 \\ \hline
    \end{tabular}
    \caption{Classification report of ResNet50 on CinC 2017}
    \label{cinc2017_clf_rp_resnet50}
\end{table}

\begin{table}[h]
    \centering
    \begin{tabular}{|l|r|r|r|r|}
    \hline
    \textbf{Classes} & \textbf{Precision} & \textbf{Recall} & \textbf{F1 Score} & \textbf{Support} \\ \hline
    N & 0.83 & 0.91 & 0.87 & 1044 \\ \hline
    A & 0.82 & 0.51 & 0.63 & 140 \\ \hline
    O & 0.72 & 0.47 & 0.57 & 473 \\ \hline
    $\sim$ & 0.00 & 0.00 & 0.00 & 49 \\ \hline
    micro avg & 0.81 & 0.73 & 0.77 & 1706 \\ \hline
    macro avg & 0.59 & 0.47 & 0.52 & 1706 \\ \hline
    weighted avg & 0.78 & 0.73 & 0.74 & 1706 \\ \hline
    samples avg & 0.73 & 0.73 & 0.73 & 1706 \\ \hline
    \end{tabular}
    \caption{Classification report of DenseNet121 on CinC 2017}
    \label{cinc2017_clf_rp_densenet121}
\end{table}

\begin{table}[h]
    \centering
    \begin{tabular}{|l|r|r|r|r|}
    \hline
    \textbf{Classes} & \textbf{Precision} & \textbf{Recall} & \textbf{F1 Score} & \textbf{Support} \\ \hline
    N & 0.88 & 0.95 & 0.91 & 1044 \\ \hline
    A & 0.78 & 0.77 & 0.77 & 140 \\ \hline
    O & 0.86 & 0.62 & 0.72 & 473 \\ \hline
    $\sim$ & 0.67 & 0.41 & 0.51 & 49 \\ \hline
    micro avg & 0.86 & 0.83 & 0.84 & 1706 \\ \hline
    macro avg & 0.8 & 0.69 & 0.73 & 1706 \\ \hline
    weighted avg & 0.86 & 0.83 & 0.84 & 1706 \\ \hline
    samples avg & 0.83 & 0.83 & 0.83 & 1706 \\ \hline
    \end{tabular}
    \caption{Classification report of 1D CNN on CinC 2017}
    \label{cinc2017_clf_rp_cnn1d}
\end{table}

\begin{table}[h]
    \centering
    \begin{tabular}{|l|r|r|r|r|}
    \hline
    \textbf{Classes} & \textbf{Precision} & \textbf{Recall} & \textbf{F1 Score} & \textbf{Support} \\ \hline
    N & 0.88 & 0.94 & 0.91 & 1044 \\ \hline
    A & 0.8 & 0.87 & 0.83 & 140 \\ \hline
    O & 0.83 & 0.69 & 0.75 & 473 \\ \hline
    $\sim$ & 0.51 & 0.51 & 0.51 & 49 \\ \hline
    micro avg & 0.85 & 0.85 & 0.85 & 1706 \\ \hline
    macro avg & 0.75 & 0.75 & 0.75 & 1706 \\ \hline
    weighted avg & 0.85 & 0.85 & 0.85 & 1706 \\ \hline
    samples avg & 0.83 & 0.85 & 0.84 & 1706 \\ \hline
    \end{tabular}
    \caption{Classification report of 1D ResNet on CinC 2017}
    \label{cinc2017_clf_rp_resnet1d}
\end{table}

\begin{table}[h]
    \centering
    \begin{tabular}{|l|r|r|r|r|}
    \hline
    \textbf{Classes} & \textbf{Precision} & \textbf{Recall} & \textbf{F1 Score} & \textbf{Support} \\ \hline
    N & 0.68 & 0.96 & 0.8 & 1044 \\ \hline
    A & 0.49 & 0.38 & 0.43 & 140 \\ \hline
    O & 0.45 & 0.66 & 0.53 & 473 \\ \hline
    $\sim$ & 0.51 & 0.61 & 0.56 & 49 \\ \hline
    micro avg & 0.60 & 0.82 & 0.69 & 1706 \\ \hline
    macro avg & 0.53 & 0.65 & 0.58 & 1706 \\ \hline
    weighted avg & 0.60 & 0.82 & 0.69 & 1706 \\ \hline
    samples avg & 0.65 & 0.82 & 0.71 & 1706 \\ \hline
    \end{tabular}
    \caption{Classification report of XGBoost on CinC 2017}
    \label{cinc2017_clf_rp_xgboost}
\end{table}

\clearpage

\section{CinC 2020}

\begin{table}[h]
    \centering
    \begin{tabular}{|l|r|r|r|r|}
    \hline
    \textbf{Classes} & \textbf{Precision} & \textbf{Recall} & \textbf{F1 Score} & \textbf{Support} \\ \hline
    AF & 0.73 & 0.68 & 0.71 & 721 \\ \hline
    AFL & 0.00 & 0.00 & 0.00 & 66 \\ \hline
    Brady & 0.00 & 0.00 & 0.00 & 58 \\ \hline
    CRBBB & 0.00 & 0.00 & 0.00 & 136 \\ \hline
    IAVB & 0.00 & 0.00 & 0.00 & 480 \\ \hline
    IRBBB & 0.00 & 0.00 & 0.00 & 294 \\ \hline
    LAD & 0.00 & 0.00 & 0.00 & 1216 \\ \hline
    LAnFB & 0.00 & 0.00 & 0.00 & 342 \\ \hline
    LBBB & 0.00 & 0.00 & 0.00 & 194 \\ \hline
    LPR & 0.00 & 0.00 & 0.00 & 62 \\ \hline
    LQRSV & 0.00 & 0.00 & 0.00 & 103 \\ \hline
    LQT & 0.00 & 0.00 & 0.00 & 301 \\ \hline
    NSIVCB & 0.00 & 0.00 & 0.00 & 201 \\ \hline
    Other & 0.62 & 0.35 & 0.45 & 4286 \\ \hline
    PAC & 0.00 & 0.00 & 0.00 & 364 \\ \hline
    PR & 0.00 & 0.00 & 0.00 & 81 \\ \hline
    PVC & 0.00 & 0.00 & 0.00 & 34 \\ \hline
    QAb & 0.00 & 0.00 & 0.00 & 206 \\ \hline
    RAD & 0.00 & 0.00 & 0.00 & 86 \\ \hline
    RBBB & 0.00 & 0.00 & 0.00 & 454 \\ \hline
    SA & 0.00 & 0.00 & 0.00 & 256 \\ \hline
    SB & 0.71 & 0.21 & 0.32 & 489 \\ \hline
    SNR & 0.64 & 0.81 & 0.72 & 4055 \\ \hline
    STach & 0.81 & 0.46 & 0.59 & 522 \\ \hline
    SVPB & 0.00 & 0.00 & 0.00 & 42 \\ \hline
    TAb & 0.00 & 0.00 & 0.00 & 918 \\ \hline
    TInv & 0.00 & 0.00 & 0.00 & 233 \\ \hline
    VPB & 0.00 & 0.00 & 0.00 & 69 \\ \hline
    micro avg & 0.65 & 0.34 & 0.45 & 16269 \\ \hline
    macro avg & 0.13 & 0.09 & 0.1 & 16269 \\ \hline
    weighted avg & 0.4 & 0.34 & 0.36 & 16269 \\ \hline
    samples avg & 0.59 & 0.4 & 0.45 & 16269 \\ \hline
    \end{tabular}
    \caption{Classification report of ResNet50 on CinC 2020}
    \label{cinc2020_clf_rp_resnet50}
\end{table}

\begin{table}[h]
    \centering
    \begin{tabular}{|l|r|r|r|r|}
    \hline
    \textbf{Classes} & \textbf{Precision} & \textbf{Recall} & \textbf{F1 Score} & \textbf{Support} \\ \hline
    AF & 0.8 & 0.72 & 0.76 & 721 \\ \hline
    AFL & 0.00 & 0.00 & 0.00 & 66 \\ \hline
    Brady & 0.00 & 0.00 & 0.00 & 58 \\ \hline
    CRBBB & 0.00 & 0.00 & 0.00 & 136 \\ \hline
    IAVB & 0.00 & 0.00 & 0.00 & 480 \\ \hline
    IRBBB & 0.00 & 0.00 & 0.00 & 294 \\ \hline
    LAD & 0.00 & 0.00 & 0.00 & 1216 \\ \hline
    LAnFB & 0.00 & 0.00 & 0.00 & 342 \\ \hline
    LBBB & 0.00 & 0.00 & 0.00 & 194 \\ \hline
    LPR & 0.00 & 0.00 & 0.00 & 62 \\ \hline
    LQRSV & 0.00 & 0.00 & 0.00 & 103 \\ \hline
    LQT & 0.00 & 0.00 & 0.00 & 301 \\ \hline
    NSIVCB & 0.00 & 0.00 & 0.00 & 201 \\ \hline
    Other & 0.59 & 0.6 & 0.59 & 4286 \\ \hline
    PAC & 0.00 & 0.00 & 0.00 & 364 \\ \hline
    PR & 0.00 & 0.00 & 0.00 & 81 \\ \hline
    PVC & 0.00 & 0.00 & 0.00 & 34 \\ \hline
    QAb & 0.00 & 0.00 & 0.00 & 206 \\ \hline
    RAD & 0.00 & 0.00 & 0.00 & 86 \\ \hline
    RBBB & 0.00 & 0.00 & 0.00 & 454 \\ \hline
    SA & 0.00 & 0.00 & 0.00 & 256 \\ \hline
    SB & 0.64 & 0.38 & 0.47 & 489 \\ \hline
    SNR & 0.66 & 0.72 & 0.69 & 4055 \\ \hline
    STach & 0.76 & 0.74 & 0.75 & 522 \\ \hline
    SVPB & 0.00 & 0.00 & 0.00 & 42 \\ \hline
    TAb & 0.00 & 0.00 & 0.00 & 918 \\ \hline
    TInv & 0.00 & 0.00 & 0.00 & 233 \\ \hline
    VPB & 0.00 & 0.00 & 0.00 & 69 \\ \hline
    micro avg & 0.64 & 0.4 & 0.5 & 16269 \\ \hline
    macro avg & 0.12 & 0.11 & 0.12 & 16269 \\ \hline
    weighted avg & 0.4 & 0.4 & 0.4 & 16269 \\ \hline
    samples avg & 0.62 & 0.47 & 0.5 & 16269 \\ \hline
    \end{tabular}
    \caption{Classification report of DenseNet121 on CinC 2020}
    \label{cinc2020_clf_rp_densenet121}
\end{table}

\begin{table}[h]
    \centering
    \begin{tabular}{|l|r|r|r|r|}
    \hline
    \textbf{Classes} & \textbf{Precision} & \textbf{Recall} & \textbf{F1 Score} & \textbf{Support} \\ \hline
    AF & 0.71 & 0.87 & 0.78 & 721 \\ \hline
    AFL & 0.00 & 0.00 & 0.00 & 66 \\ \hline
    Brady & 0.00 & 0.00 & 0.00 & 58 \\ \hline
    CRBBB & 0.65 & 0.38 & 0.48 & 136 \\ \hline
    IAVB & 0.74 & 0.52 & 0.61 & 480 \\ \hline
    IRBBB & 0.00 & 0.00 & 0.00 & 294 \\ \hline
    LAD & 0.65 & 0.66 & 0.66 & 1216 \\ \hline
    LAnFB & 0.6 & 0.78 & 0.68 & 342 \\ \hline
    LBBB & 0.85 & 0.74 & 0.79 & 194 \\ \hline
    LPR & 0.00 & 0.00 & 0.00 & 62 \\ \hline
    LQRSV & 0.00 & 0.00 & 0.00 & 103 \\ \hline
    LQT & 0.00 & 0.00 & 0.00 & 301 \\ \hline
    NSIVCB & 0.00 & 0.00 & 0.00 & 201 \\ \hline
    Other & 0.7 & 0.79 & 0.74 & 4286 \\ \hline
    PAC & 0.00 & 0.00 & 0.00 & 364 \\ \hline
    PR & 0.92 & 0.81 & 0.86 & 81 \\ \hline
    PVC & 0.00 & 0.00 & 0.00 & 34 \\ \hline
    QAb & 0.00 & 0.00 & 0.00 & 206 \\ \hline
    RAD & 0.76 & 0.3 & 0.43 & 86 \\ \hline
    RBBB & 0.86 & 0.58 & 0.69 & 454 \\ \hline
    SA & 0.00 & 0.00 & 0.00 & 256 \\ \hline
    SB & 0.61 & 0.76 & 0.67 & 489 \\ \hline
    SNR & 0.89 & 0.9 & 0.9 & 4055 \\ \hline
    STach & 0.8 & 0.8 & 0.8 & 522 \\ \hline
    SVPB & 0.00 & 0.00 & 0.00 & 42 \\ \hline
    TAb & 0.00 & 0.00 & 0.00 & 918 \\ \hline
    TInv & 0.00 & 0.00 & 0.00 & 233 \\ \hline
    VPB & 0.00 & 0.00 & 0.00 & 69 \\ \hline
    micro avg & 0.76 & 0.63 & 0.69 & 16269 \\ \hline
    macro avg & 0.35 & 0.32 & 0.32 & 16269 \\ \hline
    weighted avg & 0.61 & 0.63 & 0.62 & 16269 \\ \hline
    samples avg & 0.76 & 0.68 & 0.69 & 16269 \\ \hline
    \end{tabular}
    \caption{Classification report of 1D CNN on CinC 2020}
    \label{cinc2020_clf_rp_cnn1d}
\end{table}

\begin{table}[h]
    \centering
    \begin{tabular}{|l|r|r|r|r|}
    \hline
    \textbf{Classes} & \textbf{Precision} & \textbf{Recall} & \textbf{F1 Score} & \textbf{Support} \\ \hline
    AF & 0.83 & 0.88 & 0.86 & 721 \\ \hline
    AFL & 0.54 & 0.38 & 0.45 & 66 \\ \hline
    Brady & 0.40 & 0.21 & 0.27 & 58 \\ \hline
    CRBBB & 0.63 & 0.55 & 0.59 & 136 \\ \hline
    IAVB & 0.73 & 0.71 & 0.72 & 480 \\ \hline
    IRBBB & 0.30 & 0.1 & 0.14 & 294 \\ \hline
    LAD & 0.69 & 0.66 & 0.67 & 1216 \\ \hline
    LAnFB & 0.66 & 0.72 & 0.69 & 342 \\ \hline
    LBBB & 0.80 & 0.85 & 0.82 & 194 \\ \hline
    LPR & 0.34 & 0.34 & 0.34 & 62 \\ \hline
    LQRSV & 0.45 & 0.10 & 0.16 & 103 \\ \hline
    LQT & 0.51 & 0.45 & 0.48 & 301 \\ \hline
    NSIVCB & 0.47 & 0.11 & 0.18 & 201 \\ \hline
    Other & 0.79 & 0.69 & 0.74 & 4286 \\ \hline
    PAC & 0.62 & 0.35 & 0.45 & 364 \\ \hline
    PR & 0.92 & 0.84 & 0.88 & 81 \\ \hline
    PVC & 0.10 & 0.03 & 0.05 & 34 \\ \hline
    QAb & 0.50 & 0.02 & 0.04 & 206 \\ \hline
    RAD & 0.48 & 0.16 & 0.24 & 86 \\ \hline
    RBBB & 0.75 & 0.72 & 0.74 & 454 \\ \hline
    SA & 0.37 & 0.06 & 0.11 & 256 \\ \hline
    SB & 0.73 & 0.73 & 0.73 & 489 \\ \hline
    SNR & 0.88 & 0.91 & 0.9 & 4055 \\ \hline
    STach & 0.79 & 0.84 & 0.82 & 522 \\ \hline
    SVPB & 0.00 & 0.00 & 0.00 & 42 \\ \hline
    TAb & 0.43 & 0.29 & 0.34 & 918 \\ \hline
    TInv & 0.27 & 0.01 & 0.02 & 233 \\ \hline
    VPB & 0.41 & 0.16 & 0.23 & 69 \\ \hline
    micro avg & 0.77 & 0.66 & 0.71 & 16269 \\ \hline
    macro avg & 0.55 & 0.42 & 0.45 & 16269 \\ \hline
    weighted avg & 0.73 & 0.66 & 0.68 & 16269 \\ \hline
    samples avg & 0.77 & 0.71 & 0.71 & 16269 \\ \hline
    \end{tabular}
    \caption{Classification report of 1D ResNet on CinC 2020}
    \label{cinc2020_clf_rp_resnet1d}
\end{table}

\begin{table}[h]
    \centering
    \begin{tabular}{|l|r|r|r|r|}
    \hline
    \textbf{Classes} & \textbf{Precision} & \textbf{Recall} & \textbf{F1 Score} & \textbf{Support} \\ \hline
    AF & 0.69 & 0.57 & 0.62 & 721 \\ \hline
    AFL & 0.5 & 0.03 & 0.06 & 66 \\ \hline
    Brady & 0.26 & 0.09 & 0.13 & 58 \\ \hline
    CRBBB & 0.61 & 0.48 & 0.54 & 136 \\ \hline
    IAVB & 0.55 & 0.08 & 0.14 & 480 \\ \hline
    IRBBB & 0.23 & 0.04 & 0.07 & 294 \\ \hline
    LAD & 0.47 & 0.47 & 0.47 & 1216 \\ \hline
    LAnFB & 0.48 & 0.17 & 0.25 & 342 \\ \hline
    LBBB & 0.71 & 0.78 & 0.74 & 194 \\ \hline
    LPR & 0 & 0 & 0 & 62 \\ \hline
    LQRSV & 0.38 & 0.03 & 0.05 & 103 \\ \hline
    LQT & 0.31 & 0.13 & 0.19 & 301 \\ \hline
    NSIVCB & 0.5 & 0.02 & 0.04 & 201 \\ \hline
    Other & 0.59 & 0.89 & 0.71 & 4286 \\ \hline
    PAC & 0.51 & 0.09 & 0.15 & 364 \\ \hline
    PR & 0.94 & 0.8 & 0.87 & 81 \\ \hline
    PVC & 0.07 & 0.03 & 0.04 & 34 \\ \hline
    QAb & 0.75 & 0.03 & 0.06 & 206 \\ \hline
    RAD & 0.57 & 0.6 & 0.59 & 86 \\ \hline
    RBBB & 0.71 & 0.7 & 0.71 & 454 \\ \hline
    SA & 0.47 & 0.08 & 0.13 & 256 \\ \hline
    SB & 0.81 & 0.75 & 0.78 & 489 \\ \hline
    SNR & 0.83 & 0.94 & 0.88 & 4055 \\ \hline
    STach & 0.82 & 0.73 & 0.77 & 522 \\ \hline
    SVPB & 0 & 0 & 0 & 42 \\ \hline
    TAb & 0.39 & 0.31 & 0.35 & 918 \\ \hline
    TInv & 0.35 & 0.03 & 0.06 & 233 \\ \hline
    VPB & 0.57 & 0.06 & 0.11 & 69 \\ \hline
    micro avg & 0.66 & 0.65 & 0.65 & 16269 \\ \hline
    macro avg & 0.5 & 0.32 & 0.34 & 16269 \\ \hline
    weighted avg & 0.63 & 0.65 & 0.6 & 16269 \\ \hline
    samples avg & 0.68 & 0.69 & 0.65 & 16269 \\ \hline
    \end{tabular}
    \caption{Classification report of XGBoost on CinC 2020}
    \label{cinc2020_clf_rp_xgb}
\end{table}

\chapter{Feature Importance Index of XGBoost}

\begin{table}[h]
\begin{tabularx}{\textwidth}{|l|X|}
\hline
\textbf{Group} & \textbf{Description} \\ \hline
\texttt{fft\_coefficient} & The coefficient of 1D discrete Fourier transform \\ \hline
\texttt{ratio\_beyond\_r\_sigma} & Ratio of data that are more than $r \times \text{std}(x)$  away from the mean of x. \\ \hline
\texttt{autocorrelation} & The autocorrelation of the specified lag \\ \hline
\texttt{energy\_ratio\_by\_chunks} & The sum of squares of chunk $i$ out of $N$ chunks expressed as a ratio with the sum of squares over the whole data \\ \hline
\texttt{index\_mass\_quantile} & The relative index $i$ of data where $q\%$ of the mass of data lies left of $i$ \\ \hline
\texttt{lempel\_ziv\_complexity} & Complexity estimate from Lempel-Ziv algorithm \\ \hline
\texttt{agg\_autocorrelation} & Descriptive statistics on the autocorrelation of data \\ \hline
\texttt{range\_count} & The number of item within the interval \\ \hline
\texttt{spkt\_welch\_density} & The cross power spectral density of data \\ \hline
\texttt{change\_quantiles} & The average, absolute value of consecutive changes of data inside a specific corridor \\ \hline
\texttt{quantile} & A specific quantile of data \\ \hline
\texttt{number\_peaks} & The number of peaks of at least support a threshold in the data \\ \hline
\texttt{count\_below} & Percentage of data lower than a threshold \\ \hline
\texttt{cwt\_coefficients} & The Continuous wavelet transform for the Ricker wavelet \\ \hline
\texttt{number\_crossing\_m} & The number of crossings in data over a specific threshold \\ \hline
\texttt{maximum} & The maximum of data \\ \hline
\texttt{kurtosis} & The Kurtosis of data \\ \hline
\texttt{skewness} & The Skewness of data \\ \hline
\texttt{fft\_aggregated} & Descriptive statistics of the absolute Fourier transform spectrum \\ \hline
\texttt{benford\_correlation} & The correlation from the first digit distribution \\ \hline
\texttt{binned\_entropy} & The entropy after binning data \\ \hline
\texttt{count\_above} & Percentage of data higher than a threshold \\ \hline
\end{tabularx}
\caption{Description of each feature group in XGBoost model.}
\label{tab:ft_group_des}
\end{table}
